# Supplementary material for: Filling the Gaps in Ancient Akkadian Texts: A Masked Language Modelling Approach
Source: arXiv:2109.04513 source file (2021-10-24)
Supplement: Supplementary file 1 [file appendix.tex]

\korenl{a detailed description of the models' hyperparameters (including M-BERT added head}
